# Supplementary material for: Direct unconstrained optimization of excited states in density functional theory
Source: arXiv:2501.10907 source file (2025-01-19)
Supplement: Supplementary file 1 [file SI.pdf]

## Supporting Information for:
## Direct unconstrained optimization of excited states in density functional theory

Hanh D. M. Pham and Rustam Z. Khaliullin
*Department of Chemistry, McGill University, 801 Sherbrooke St West, Montreal, QC H3A 0B8, Canada*

Email: rustam.khaliullin@mcgill.ca

### I. KEY EQUATIONS AND THEIR DERIVATION

#### A. Unrestricted Kohn Sham equations for variable metric time-independent optimization

In the unrestricted Kohn-Sham (UKS) method, molecular orbital coefficients for different spins are optimized independently. The notation and definitions are described in the main text. The Kohn-Sham energy functional and the electron density are given by

$$E^I = \sum_{\tau=\alpha}^{\beta}\sum_{\mu\nu}^{B} F_{\mu\nu}^{I\tau} P_{\nu\mu}^{I\tau} - \frac{1}{2}\int\int \frac{\rho^I(\mathbf{r})\rho^I(\mathbf{r}')}{|\mathbf{r}-\mathbf{r}'|} d\mathbf{r}d\mathbf{r}' + E_{xc}^I - \int \upsilon_{XC}^I(\mathbf{r})\rho^I(\mathbf{r})d\mathbf{r} \tag{1}$$

$$\rho^{I\tau}(\mathbf{r}) = \sum_{ij=1}^{N} \phi_i^{I\tau *}(\mathbf{r})(\sigma_{I\tau}^{-1})_{ij}\phi_j^{I\tau}(\mathbf{r}) = \sum_{\mu\nu=1}^{B} \chi_\mu^*(\mathbf{r}) P_{\mu\nu}^{I\tau}\chi_\nu(\mathbf{r}) \tag{2}$$

#### B. First derivative of the intrastate term

The derivation of the intrastate term is presented in the Supporting Information of our previous work[?] .

$$\begin{aligned} G_{\mu i}^{I\tau\mathcal{E}} &\equiv \frac{\partial \mathcal{E}^I}{\partial T_{\mu i}^{I\tau}} = \frac{\partial E^I}{\partial T_{\mu i}^{I\tau}} - \sum_{\tau=\alpha}^{\beta}\left[c_p^I \frac{\partial \ln\det\left(\sigma_{II\tau}\sigma_{II\tau d}^{-1}\right)}{\partial T_{\mu i}^{I\tau}}\right] = \\ &= 2[(I - SP^{I\tau})F^{I\tau}T^{I\tau}(\sigma_{II\tau}^{-1})]_{\mu i} - 2c_p^I[ST^{I\tau}(\sigma_{II\tau}^{-1} - \sigma_{II\tau d}^{-1})]_{\mu i} \end{aligned} \tag{3}$$

#### C. First derivative of the interstate term

The first derivative of the interstate penalty term is

$$\begin{aligned} G_{\mu i}^{I\tau P} &= \frac{\partial \Omega_P}{\partial T_{\mu i}^{I\tau}} = -C_P \sum_{\tau'=\alpha,\beta} \delta_{\tau\tau'} \frac{\partial \ln[\det(\Phi_{\tau'}\Phi_{\tau' d}^{-1})]}{\partial T_{\mu i}^{I\tau}} = \\ &= -C_P \frac{1}{\det(\Phi_\tau \Phi_{\tau d}^{-1})} \frac{\partial\left[\det(\Phi_\tau)\det(\Phi_{\tau d}^{-1})\right]}{\partial T_{\mu i}^{I\tau}} = \\ &= -C_P \frac{1}{\det(\Phi_\tau \Phi_{\tau d}^{-1})}\left[\frac{\partial \det(\Phi_\tau)}{\partial T_{\mu i}^{I\tau}}\det(\Phi_{\tau d}^{-1}) + \det(\Phi_\tau)\frac{\partial\left[\det(\Phi_{\tau d})\right]^{-1}}{\partial \det(\Phi_{\tau d})}\frac{\partial \det(\Phi_{\tau d})}{\partial T_{\mu i}^{I\tau}}\right] = \\ &= -C_P\left[\frac{1}{\det(\Phi_\tau)}\frac{\partial \det(\Phi_\tau)}{\partial T_{\mu i}^{I\tau}} - \frac{1}{\det(\Phi_{\tau d})}\frac{\partial \det(\Phi_{\tau d})}{\partial T_{\mu i}^{I\tau}}\right] \end{aligned} \tag{4}$$

The derivative in the first term is evaluated using the fact that $\Phi$ is an invertible matrix, but matrices $\sigma_{IJ\tau}$ matrices are not necessarily invertible

$$
\begin{aligned}
\frac{\partial \det(\Phi_\tau)}{\partial T^{I\tau}_{\mu i}} &= \det(\Phi_\tau)\sum_{KJ}(\Phi_\tau^{-1})_{KJ}\frac{\partial \Phi_{\tau JK}}{\partial T^{I\tau}_{\mu i}} = \det(\Phi_\tau)\sum_{KJ}(\Phi_\tau^{-1})_{KJ}\frac{\partial \det(\sigma_{JK\tau})}{\partial T^{I\tau}_{\mu i}} = \\
&= \det(\Phi_\tau)\sum_{KJ}(\Phi_\tau^{-1})_{KJ}\sum_{jk}\mathrm{adj}(\sigma_{JK\tau})_{kj}\frac{\partial(\sum_{\alpha\lambda}T^{J\tau}_{\lambda j}S_{\lambda\alpha}T^{K\tau}_{\alpha k})}{\partial T^{I\tau}_{\mu i}} = \\
&= \det(\Phi_\tau)\sum_{KJ}(\Phi_\tau^{-1})_{KJ}\sum_{jk}\mathrm{adj}(\sigma_{JK\tau})_{kj}(\sum_{\alpha\lambda}\frac{\partial T^{J\tau}_{\lambda j}}{T^{I\tau}_{\mu i}}S_{\lambda\alpha}T^{K\tau}_{\alpha k} + \sum_{\alpha\lambda}T^{J\tau}_{\lambda j}S_{\lambda\alpha}\frac{\partial T^{K\tau}_{\alpha k}}{T^{I\tau}_{\mu i}}) = \\
&= \det(\Phi_\tau)\sum_{KJ}(\Phi_\tau^{-1})_{KJ}\sum_{jk}\mathrm{adj}(\sigma_{JK\tau})_{kj}(\sum_{\alpha\lambda}\delta_{JI}\delta_{\lambda\mu}\delta_{ji}S_{\lambda\alpha}T^{K\tau}_{\alpha k} + \sum_{\alpha\lambda}T^{J\tau}_{\lambda j}S_{\lambda\alpha}\delta_{KI}\delta_{\alpha\mu}\delta_{ki}) = \\
&= \det(\Phi_\tau)\sum_{KJ}(\Phi_\tau^{-1})_{KJ}\sum_{jk}\mathrm{adj}(\sigma_{JK\tau})_{kj}[\delta_{JI}\delta_{ji}(ST^{K\tau})_{\mu k} + (T^{J\tau\dagger}S)_{j\mu}\delta_{KI}\delta_{ki}] = \\
&= \det(\Phi_\tau)[\sum_{Kk}(\Phi_\tau^{-1})_{KI}\,\mathrm{adj}(\sigma_{IK\tau})_{ki}(ST^{K\tau})_{\mu k} + \sum_{Jj}(\Phi_\tau^{-1})_{IJ}\,\mathrm{adj}(\sigma_{JI\tau})_{ij}(T^{J\tau\dagger}S)_{j\mu}] = \\
&= \det(\Phi_\tau)[\sum_{K}(\Phi_\tau^{-1})_{KI}[ST^{K\tau}\mathrm{adj}(\sigma_{IK\tau})]_{\mu i} + \sum_{J}(\Phi_\tau^{-1})_{IJ}[\mathrm{adj}(\sigma_{JI\tau})T^{J\tau\dagger}S]_{i\mu}] = \\
&= 2\det(\Phi_\tau)\sum_{K}(\Phi_\tau^{-1})_{KI}[ST^{K\tau}\mathrm{adj}(\sigma_{IK\tau})]_{\mu i}
\end{aligned}
\tag{5}
$$

The derivative in the second term can be obtained using the result for the first term, the fact that $\Phi_{\tau d}$ is a diagonal matrix, and that $\sigma_{II\tau}$ is invertible with $\mathrm{adj}(\sigma_{II\tau}) = \det(\sigma_{II\tau})(\sigma^{-1}_{II\tau})$ for an invertible matrix:

$$
\begin{aligned}
\frac{\partial \det(\Phi_{\tau d})}{\partial T^{I\tau}_{\mu i}} &= 2\det(\Phi_{\tau d})\sum_{K}(\Phi^{-1}_{\tau d})_{KI}[ST^{K\tau}\mathrm{adj}(\sigma_{IK\tau d})]_{\mu i} = \\
&= 2\det(\Phi_{\tau d})(\Phi^{-1}_{\tau d})_{II}[ST^{I\tau}\mathrm{adj}(\sigma_{II\tau})]_{\mu i} = \\
&= 2\det(\Phi_{\tau d})[\det(\sigma_{II\tau})]^{-1}[ST^{I\tau}\det(\sigma_{II\tau})(\sigma^{-1}_{II\tau})]_{\mu i} = \\
&= 2\det(\Phi_{\tau d})[ST^{I\tau}(\sigma^{-1}_{II\tau})]_{\mu i}
\end{aligned}
\tag{6}
$$

Using these results the first derivative of the interstate penalty term is

$$
G^{I\tau P}_{\mu i} = -2C_P\left[\sum_{K}(\Phi_\tau)^{-1}_{IK}\left[ST^{K\tau}\mathrm{adj}(\sigma_{IK\tau})\right]_{\mu i} - (ST^{I\tau}\sigma^{-1}_{II\tau})_{\mu i}\right]
\tag{7}
$$
